# Supplementary material for: VOEvent Standard for Fast Radio Bursts
Source: arXiv:1710.08155 ancillary file (2017-10-23)
Supplement: Supplementary file 1 [file parameter_table.pdf]

Table 1: Parameter descriptions for the elements and groups within an FRB VOEvent including information on whether the parameter is required (✓) or optional (○) within the different event types: 1 - Detection, 2 - Subsequent, 3 - Update, 4 - Retraction, I - Search, II - Targeted.

| Element                | Group                  | Parameter            | Included in |   |   |   |   |                                                                                                                                                                                                | Description and Notes                                                                                                    |
|------------------------|------------------------|----------------------|-------------|---|---|---|---|------------------------------------------------------------------------------------------------------------------------------------------------------------------------------------------------|--------------------------------------------------------------------------------------------------------------------------|
|                        |                        |                      | 1           | 2 | 3 | 4 | I | II                                                                                                                                                                                             |                                                                                                                          |
| Header                 |                        | role                 | ✓           | ✓ | ✓ | ✓ | ✓ | ✓                                                                                                                                                                                              | <i>observation</i> (Detection, Subsequent, Update, Retraction),<br><i>utility</i> (Search, Targeted), or <i>test</i>     |
| <Who>                  | Observatory parameters | Event IVORN          | ✓           | ✓ | ✓ | ✓ | ✓ | ✓                                                                                                                                                                                              | A unique identifier for the VOEvent                                                                                      |
|                        |                        | Author IVORN         | ✓           | ✓ | ✓ | ✓ | ✓ | ✓                                                                                                                                                                                              | An identifier for the author in the same format as the Event IVORN                                                       |
|                        |                        | Date                 | ✓           | ✓ | ✓ | ✓ | ✓ | ✓                                                                                                                                                                                              | Time of the event creation                                                                                               |
|                        |                        | Author               | ✓           | ✓ | ✓ | ✓ | ✓ | ✓                                                                                                                                                                                              | Author contact e-mail and name                                                                                           |
| <What>                 |                        | beam_semi-major_axis | ✓           | ✓ | ○ |   | ✓ | ✓                                                                                                                                                                                              | Semi-major axis of the detection beam in arcminutes.                                                                     |
|                        |                        | beam_semi-minor_axis | ✓           | ✓ | ○ |   | ✓ | ✓                                                                                                                                                                                              | Semi-minor axis of the detection beam in arcminutes.                                                                     |
|                        |                        | rotation_angle       | ✓           | ✓ | ○ |   | ✓ | ✓                                                                                                                                                                                              | Rotation angle of the beam with respect to Right<br>Ascension (RA) in degrees.                                           |
|                        |                        | sampling_time        | ✓           | ✓ | ○ |   | ✓ | ✓                                                                                                                                                                                              | Sampling time of the datataking instrument in milliseconds.                                                              |
|                        |                        | bandwidth            | ✓           | ✓ | ○ |   | ✓ | ✓                                                                                                                                                                                              | Frequency bandwidth of the datataking instrument in MHz.                                                                 |
|                        |                        | nchan                | ✓           | ✓ | ○ |   | ✓ | ✓                                                                                                                                                                                              | Number of frequency channels across the observing bandwidth.                                                             |
|                        |                        | centre_frequency     | ✓           | ✓ | ○ |   | ✓ | ✓                                                                                                                                                                                              | Centre observing frequency of the datataking instrument in MHz.                                                          |
|                        |                        | npol                 | ✓           | ✓ | ○ |   | ✓ | ✓                                                                                                                                                                                              | Number of polarisations of the datataking instrument.                                                                    |
|                        |                        | bits_per_sample      | ✓           | ✓ | ○ |   | ✓ | ✓                                                                                                                                                                                              | Number of bits per sample of the datataking instrument.                                                                  |
|                        |                        | gain                 | ✓           | ✓ | ○ |   | ✓ | ✓                                                                                                                                                                                              | Telescope instrument gain in K/Jy.                                                                                       |
|                        |                        | tsys                 | ✓           | ✓ | ○ |   | ✓ | ✓                                                                                                                                                                                              | Telescope instrument system temperature in K.                                                                            |
|                        |                        | backend              | ✓           | ✓ | ○ |   | ✓ | ✓                                                                                                                                                                                              | Name of the datataking instrument (e.g. BPSR, GUPPI).                                                                    |
|                        |                        | beam                 | ✓           | ✓ | ○ |   | ✓ | ✓                                                                                                                                                                                              | Number or designation of the detection beam, if applicable.                                                              |
| Observation parameters | observation_start_MJD  |                      |             |   |   | ✓ | ✓ | The MJD start time of the planned observation.                                                                                                                                                 |                                                                                                                          |
|                        | observation_end_MJD    |                      |             |   |   | ✓ | ✓ | The MJD end time of the planned observation.                                                                                                                                                   |                                                                                                                          |
|                        | observation_duration   |                      |             |   |   | ✓ | ✓ | The duration of the planned observation.                                                                                                                                                       |                                                                                                                          |
|                        | observation_RA         |                      |             |   |   | ✓ | ✓ | The RA position of the boresight of the primary beam.                                                                                                                                          |                                                                                                                          |
|                        | observation_DEC        |                      |             |   |   | ✓ | ✓ | The Dec position of the boresight of the primary beam.                                                                                                                                         |                                                                                                                          |
|                        | target_name            |                      |             |   |   |   | ✓ | The name of the planned target (e.g. FRB 121102) for the Targeted type.<br>If no VOEvent citation exists for this event, provide the DOI of the FRB<br>publication in the Description element. |                                                                                                                          |
|                        | scan_type              |                      |             |   |   | ✓ |   | Options: “Fixed” or “Drift”. Only used with the Search element.                                                                                                                                |                                                                                                                          |
|                        | Event parameters       | dm                   | ✓           | ✓ | ○ |   |   |                                                                                                                                                                                                | The best-fit dispersion measure of the FRB in pc cm <sup>−3</sup> .                                                      |
|                        |                        | dm_error             | ✓           | ✓ | ○ |   |   |                                                                                                                                                                                                | The error on the best-fit dispersion measure in pc cm <sup>−3</sup> .                                                    |
|                        |                        | width                | ✓           | ✓ | ○ |   |   |                                                                                                                                                                                                | The width (or duration) of the pulse in milliseconds.                                                                    |
|                        |                        | snr                  | ✓           | ✓ | ○ |   |   |                                                                                                                                                                                                | The signal-to-noise ratio of the detected pulse.                                                                         |
|                        |                        | flux                 | ✓           | ✓ | ○ |   |   |                                                                                                                                                                                                | The peak flux density of the radio pulse in Janskys. Specify in the parameter<br>description how the flux is determined. |
|                        |                        | gl                   | ✓           | ✓ | ○ |   |   |                                                                                                                                                                                                | The Galactic longitude in degrees.                                                                                       |
| gb                     |                        | ✓                    | ✓           | ○ |   |   |   | The Galactic latitude in degrees.                                                                                                                                                              |                                                                                                                          |

| Element | Group               | Parameter               | Included in           |                       |                       |   |   |    | Description and Notes                                                                                                                                                                                                                                                                                                                                             |
|---------|---------------------|-------------------------|-----------------------|-----------------------|-----------------------|---|---|----|-------------------------------------------------------------------------------------------------------------------------------------------------------------------------------------------------------------------------------------------------------------------------------------------------------------------------------------------------------------------|
|         |                     |                         | 1                     | 2                     | 3                     | 4 | I | II |                                                                                                                                                                                                                                                                                                                                                                   |
| <What>  | Advanced parameters | MW_dm_limit             | <input type="radio"/> | <input type="radio"/> | <input type="radio"/> |   |   |    | The modeled integrated Milky Way dispersion measure along the line of sight in $\text{pc cm}^{-3}$ .                                                                                                                                                                                                                                                              |
|         |                     | galactic_electron_model | <input type="radio"/> | <input type="radio"/> | <input type="radio"/> |   |   |    | The name of the model used to estimate the Galactic dispersion measure contribution. Fixed options available for this parameter include “NE2001”, “TC93”, “YMW16”, and “Other”. If “Other” is used, please specify DOI or description of model in the Description element.                                                                                        |
|         |                     | redshift_inferred       | <input type="radio"/> | <input type="radio"/> | <input type="radio"/> |   |   |    | The inferred redshift estimated based on e.g. the dispersion measure. Specify method of calculation in the Description element.                                                                                                                                                                                                                                   |
|         |                     | redshift_host           | <input type="radio"/> | <input type="radio"/> | <input type="radio"/> |   |   |    | The redshift of the FRB host galaxy. Specify “photometry” or “spectroscopy” in the Description element.                                                                                                                                                                                                                                                           |
|         |                     | dispersion_smearing     | <input type="radio"/> | <input type="radio"/> | <input type="radio"/> |   |   |    | The intrachannel smearing of the pulse due to channel width and dispersion measure in milliseconds.                                                                                                                                                                                                                                                               |
|         |                     | scattering              | <input type="radio"/> | <input type="radio"/> | <input type="radio"/> |   |   |    | The scatter broadening of the pulse due to scattering in milliseconds. A value of “None” here could mean either that no scattering has been detected or that a measurement/fit has not been made.                                                                                                                                                                 |
|         |                     | scattering_model        | <input type="radio"/> | <input type="radio"/> | <input type="radio"/> |   |   |    | Scattering screen model used to measure scattering parameter. Value is any of the following options: “one-sided exponential”(standard), “Kolmogorov thin screen”, “Kolmogorov uniform medium”, “Kolmogorov thin-screen truncated”, “Power law thin”, “Power law thick”, “other”. In case of “other”, specify the method that was used in the Description element. |
|         |                     | dm_index                | <input type="radio"/> | <input type="radio"/> | <input type="radio"/> |   |   |    | The dispersion measure index of the FRB.                                                                                                                                                                                                                                                                                                                          |
|         |                     | dm_index_error          | <input type="radio"/> | <input type="radio"/> | <input type="radio"/> |   |   |    | The error on the dispersion measure index of the FRB.                                                                                                                                                                                                                                                                                                             |
|         |                     | scattering_timescale    | <input type="radio"/> | <input type="radio"/> | <input type="radio"/> |   |   |    | The scattering timescale modeled along the line of sight at 1 GHz in ms.                                                                                                                                                                                                                                                                                          |
|         |                     | scatter_index           | <input type="radio"/> | <input type="radio"/> | <input type="radio"/> |   |   |    | The scattering index of the FRB.                                                                                                                                                                                                                                                                                                                                  |
|         |                     | scatter_index_error     | <input type="radio"/> | <input type="radio"/> | <input type="radio"/> |   |   |    | The error on the scattering index of the FRB.                                                                                                                                                                                                                                                                                                                     |
|         |                     | spectral_index          | <input type="radio"/> | <input type="radio"/> | <input type="radio"/> |   |   |    | The spectral index of the FRB.                                                                                                                                                                                                                                                                                                                                    |
|         |                     | spectral_index_error    | <input type="radio"/> | <input type="radio"/> | <input type="radio"/> |   |   |    | The error on the spectral index of the FRB.                                                                                                                                                                                                                                                                                                                       |
|         |                     | width_error_upper       | <input type="radio"/> | <input type="radio"/> | <input type="radio"/> |   |   |    | The upper error on the measured width of the FRB in ms.                                                                                                                                                                                                                                                                                                           |
|         |                     | width_error_lower       | <input type="radio"/> | <input type="radio"/> | <input type="radio"/> |   |   |    | The lower error on the measured width of the FRB in ms.                                                                                                                                                                                                                                                                                                           |
|         |                     | flux_calibrated         | <input type="radio"/> | <input type="radio"/> | <input type="radio"/> |   |   |    | The peak flux density in Janskys measured using instrument calibration. If this value is given the calibration method must be provided in the Description element.                                                                                                                                                                                                |
|         |                     | flux_error_upper        | <input type="radio"/> | <input type="radio"/> | <input type="radio"/> |   |   |    | The upper error on the measured flux density of the FRB in Janskys.                                                                                                                                                                                                                                                                                               |
|         |                     | flux_error_lower        | <input type="radio"/> | <input type="radio"/> | <input type="radio"/> |   |   |    | The lower error on the measured flux density of the FRB in Janskys.                                                                                                                                                                                                                                                                                               |
|         |                     | fluence                 | <input type="radio"/> | <input type="radio"/> | <input type="radio"/> |   |   |    | The fluence of the FRB in Jansky milliseconds.                                                                                                                                                                                                                                                                                                                    |
|         |                     | fluence_error_upper     | <input type="radio"/> | <input type="radio"/> | <input type="radio"/> |   |   |    | The upper error on the fluence in Jansky milliseconds.                                                                                                                                                                                                                                                                                                            |
|         |                     | fluence_error_lower     | <input type="radio"/> | <input type="radio"/> | <input type="radio"/> |   |   |    | The lower error on the fluence in Jansky milliseconds.                                                                                                                                                                                                                                                                                                            |
|         |                     | linear_pol              | <input type="radio"/> | <input type="radio"/> | <input type="radio"/> |   |   |    | The linear polarization fraction of the FRB.                                                                                                                                                                                                                                                                                                                      |
|         |                     | linear_pol_error        | <input type="radio"/> | <input type="radio"/> | <input type="radio"/> |   |   |    | The error on the linear polarization fraction of the FRB.                                                                                                                                                                                                                                                                                                         |
|         |                     | circular_pol            | <input type="radio"/> | <input type="radio"/> | <input type="radio"/> |   |   |    | The circular polarization fraction of the FRB.                                                                                                                                                                                                                                                                                                                    |
|         |                     | circular_pol_error      | <input type="radio"/> | <input type="radio"/> | <input type="radio"/> |   |   |    | The error on the circular polarization fraction of the FRB.                                                                                                                                                                                                                                                                                                       |
|         |                     | rm                      | <input type="radio"/> | <input type="radio"/> | <input type="radio"/> |   |   |    | The rotation measure of the FRB in radians $\text{m}^{-2}$ .                                                                                                                                                                                                                                                                                                      |
|         |                     | rm_error                | <input type="radio"/> | <input type="radio"/> | <input type="radio"/> |   |   |    | The error on the rotation measure in radians $\text{m}^{-2}$ .                                                                                                                                                                                                                                                                                                    |

| Element     | Group | Parameter           | Included in |   |   |   |   |    | Description and Notes                                                                                                                                                                                                                                                                                                                                                                                                                                                 |
|-------------|-------|---------------------|-------------|---|---|---|---|----|-----------------------------------------------------------------------------------------------------------------------------------------------------------------------------------------------------------------------------------------------------------------------------------------------------------------------------------------------------------------------------------------------------------------------------------------------------------------------|
|             |       |                     | 1           | 2 | 3 | 4 | I | II |                                                                                                                                                                                                                                                                                                                                                                                                                                                                       |
| <WhereWhen> |       | ObservatoryLocation | ✓           | ✓ |   |   | ✓ | ✓  | The location of the observatory, either from a registry or with coordinates input manually in latitude (deg), longitude (deg), and elevation (m).                                                                                                                                                                                                                                                                                                                     |
|             |       | Time                | ✓           | ✓ | ○ |   | ✓ | ✓  | The time the FRB occurred in the format YYYY-MM-DDThh:mm:ss.ssssss to whatever precision the arrival time is known.                                                                                                                                                                                                                                                                                                                                                   |
|             |       | Position2D          | ✓           | ✓ | ○ |   | ✓ | ✓  | The RA (entry C1) and Dec (entry C2) coordinates of the FRB as well as the radius of the error circle on the position, all given in units of degrees. Note: for elliptical beams this is an imperfect position description; however, the length of the semi-major axis of the error ellipse should be used as the radius.                                                                                                                                             |
| <How>       |       |                     | ○           | ○ | ○ | ○ | ○ | ○  | Description elements can be used here to provide links to instrument details or public data repositories.                                                                                                                                                                                                                                                                                                                                                             |
| <Why>       |       | importance          | ✓           | ✓ | ✓ | ✓ | ✓ | ✓  | The importance of an event between 0 and 1, with higher importance scores corresponding to more confidence in the event. Each survey or team may have a different scoring scale for the events detected through their searches but some elaboration on the criteria used to derive the score should be given, if possible, in the description entry in the <Why> element. Importance for Update, Retraction, Search, and Targeted types should be set to 0 or “None”. |
| <Citations> |       | Name                | ✓           | ○ | ○ | ○ |   |    | The name of the FRB event in the format FRBYMMDD.                                                                                                                                                                                                                                                                                                                                                                                                                     |
|             |       | EventIVORN          |             | ✓ | ✓ | ✓ |   | ○  | The IVORN of the previous event being cited. Detection, Subsequent, and Search event types can be cited here.                                                                                                                                                                                                                                                                                                                                                         |
